# Supplementary material for: Electric fields and substrates dramatically accelerate spin relaxation in graphene
Source: arXiv:2012.11550 source file (2022-03-16)
Supplement: Supplementary file 1 [file SI.pdf]

# Supplemental material for: 'Electric field and substrate effects dominate spin-phonon relaxation in graphene'

Adela Habib,<sup>1,\*</sup> Junqing Xu,<sup>2,\*</sup> Yuan Ping,<sup>2,†</sup> and Ravishankar Sundararaman<sup>1,3,‡</sup>

<sup>1</sup>Department of Physics, Applied Physics and Astronomy, Rensselaer Polytechnic Institute, Troy, NY 12180, USA

<sup>2</sup>Department of Chemistry and Biochemistry, University of California, Santa Cruz, CA 95064, USA

<sup>3</sup>Department of Materials Science and Engineering, Rensselaer Polytechnic Institute, Troy, NY 12180, USA

(Dated: December 21, 2020)

In the *ab initio* prediction of spin-phonon relaxation times in graphene presented in the main text, the computational workflow involves the following steps. First, we perform density-functional theory (DFT) calculations of the electronic structure, phonon and electron-phonon matrix elements using the Perdew-Burke-Ernzerhof exchange-correlation functional<sup>1</sup> in the open-source plane-wave code - JDFTx.<sup>2</sup> We use fully-relativistic norm-conserving pseudopotentials<sup>3</sup> to include spin-orbit coupling self-consistently, and correspondingly use a kinetic energy cutoff of 37 Hartrees (1000 eV) for the plane-wave basis.

All calculations are performed using fully-relaxed lattice constants and internal geometries, summarized in Table I. To capture van-der-Waals interactions in the equilibrium geometry, we use the DFT+D2 correction method,<sup>4</sup> with a scale factor of 0.5 appropriate for graphene heterostructures.<sup>5</sup> For the graphene on hexagonal boron nitride (hBN) specifically, we find the AB stacking where N is positioned in the hexagonal void of graphene and B moves towards the C atom, consistent with previous studies.<sup>6</sup> This lowest energy configuration of the structure gives a spacing of 3.28 Å between graphene and hBN, in agreement with previous predictions.<sup>7</sup>

TABLE I. Converged geometry parameters for calculations.

| System       | $a$ [Å] | Vacuum spacing [Å] |
|--------------|---------|--------------------|
| Graphene     | 2.465   | 13.22              |
| Graphene/hBN | 2.486   | 13.22              |

The DFT calculations are done on ‘coarse’ electronic  $\mathbf{k}$ -meshes of  $24 \times 24 \times 1$  and phonon  $\mathbf{q}$ -meshes of  $6 \times 6 \times 1$ . We transform all the DFT computed properties to maximally localized Wannier function basis<sup>8</sup>, which provides a robust interpolation scheme to finer meshes of  $864 \times 864 \times 1$  for both  $\mathbf{k}$  and  $\mathbf{q}$  for the spin evolution simulations.<sup>9–12</sup>

To simulate the dynamics, we first prepare the initial spin states for a particular Cartesian direction by equilibrating to a small perturbation magnetic field (e.g. 1 Tesla) in that direction, removing that magnetic field at  $t = 0$  and then let the spins evolve over time. Figure 1 shows an example of in-plane and out-of-plane spin

expectation evolution over time in graphene on hBN. The relaxation times are extracted by fitting  $S_i(t) = S_i(0)e^{-t/\tau_i^s} \cos(\omega t)$ , where the  $\tau_i^s$  is the spin relaxation lifetime for Cartesian coordinates,  $i = x, y, z$ , and  $\omega$  is an oscillation frequency related to energy splitting in the band structure. In all three cases presented in this paper, we find the oscillation periods much longer than spin-relevant lifetimes which is expected because the splittings are very small in band structure. This results to mostly exponentially decaying profiles of the spin expectation values. To get a substantial decay of the spin-expectation values, e.g.,  $> 50\%$ , for reliable extraction of the spin lifetimes, the simulation time varies based on the system. Specifically, depending on the final observed relaxation time, we required simulation times ranging from 500 ps to a few  $\mu\text{s}$ .

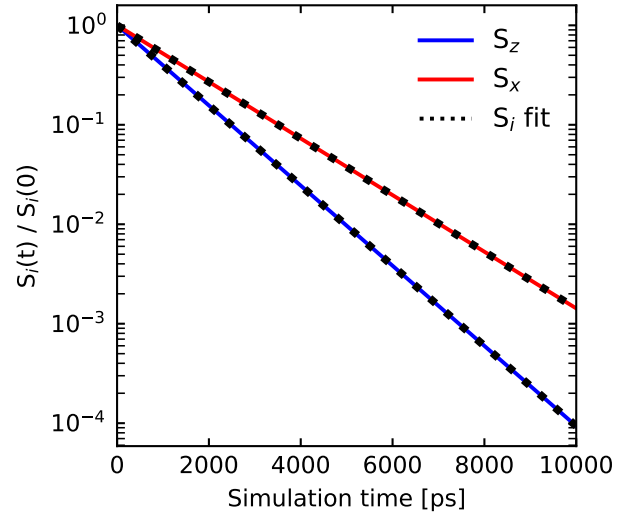

FIG. 1. Characteristic real-time evolution of the in-plane and out-of-plane spin expectation values and corresponding fits to extract spin relaxation time, shown here for graphene on hBN under zero applied electric field and an electron density of  $1.2 \times 10^{12} \text{ cm}^{-2}$ .

The energy-conserving  $\delta$ -function in Eq. 1 of the main text is implemented as a Gaussian with a finite standard deviation  $\sigma$ . We have conducted extensive convergence tests to determine the impact of this width on lifetimes and have found that for  $\sigma$  in the range of  $0.0025 - 0.005 \text{ eV}$ , the spin relaxation lifetimes change by less than  $\sim 1\%$ . For all calculations presented in the main text, we set  $\sigma = 0.005 \text{ eV}$ .

\* These authors contributed equally

† yuanping@ucsc.edu

‡ sundar@rpi.edu

For studying the impact of an applied transverse electric field on spin-phonon times, we have implemented the applied field as a Stark perturbation Hamiltonian in the Wannier basis. Specifically, we add the term

$H_{\text{Stark}} = |e|E_z z_{nn'}^k$ , to the Hamiltonian of the system in Wannier basis, where  $|e|$  is electron(hole) charge (1 in atomic units),  $E_z$  is the magnitude of electric field, and  $z_{nn'}^k$  is the matrix element of  $z$  from the DFT calculation.

- 
- [1] J. P. Perdew, K. Burke, and M. Ernzerhof, *Phys. Rev. Lett.* **77**, 3865 (1996).
  - [2] R. Sundararaman, K. Letchworth-Weaver, K. A. Schwarz, D. Gunceler, Y. Ozhabes, and T. Arias, *SoftwareX* **6**, 278 (2017).
  - [3] M. Van Setten, M. Giantomassi, E. Bousquet, M. J. Verstraete, D. R. Hamann, X. Gonze, and G.-M. Rignanese, *Comput. Phys. Commun.* **226**, 39 (2018).
  - [4] S. Grimme, *Journal of Computational Chemistry* **27**, 1787 (2006).
  - [5] P. Narang, L. Zhao, S. Claybrook, and R. Sundararaman, *Adv. Opt. Mater.* **5**, 1600914 (2017).
  - [6] J. Wang, F. Ma, and M. Sun, *RSC Adv.* **7**, 16801 (2017).
  - [7] Y. Fan, M. Zhao, Z. Wang, X. Zhang, and H. Zhang, *Applied Physics Letters* **98**, 083103 (2011).
  - [8] N. Marzari and D. Vanderbilt, *Phys. Rev. B* **56**, 12847 (1997).
  - [9] F. Giustino, M. L. Cohen, and S. G. Louie, *Phys. Rev. B* **76**, 165108 (2007).
  - [10] A. M. Brown, R. Sundararaman, P. Narang, W. A. Goddard, and H. A. Atwater, *ACS Nano* **10**, 957 (2016).
  - [11] A. M. Brown, R. Sundararaman, P. Narang, A. M. Schwartzberg, W. A. Goddard III, and H. A. Atwater, *Phys. Rev. Lett.* **118**, 087401 (2017).
  - [12] A. Habib, R. Florio, and R. Sundararaman, *J. Opt.* **20**, 064001 (2018).
